# Supplementary material for: A Simple yet Effective Self-Debiasing Framework for Transformer Models
Source: arXiv:2306.01907 source file (2023-06-02)
Supplement: Supplementary file 1 [file appendix.tex]

%\subsection{Analysis}
%\label{ssec:result-analysis}
To deeply understand the superiority of our proposed framework, we conduct more analysis to answer the following problems: 1) 
% Dose our framework performs better because it captures the right evidences?  
Dose our proposed model acquire better interpretability?
2) Is our model robust?  and 3) How dose the residual connection take effects during training?
% in terms of the interpretability, robustness, and function of model.

\paragraph{Interpretability Analysis} To further analyze the effect of model debiasing for interpretability, we evaluate the interpretability of the model from the perspectives of plausibility and faithfulness on the annotated datasets released by \cite{wang2022fine}. To this end, we introduce the following commonly-used interpretable metrics.

Note that \textbf{Token-F1} is mainly used to evaluate the model plausibility and  \textbf{sufficiency (Suff)}, \textbf{comprehensive (Comp)} and \textbf{Mean Average Precision (MAP)} are used to quantify the faithfulness.
\begin{itemize}
    \item \textbf{Token-F1} is computed by overlapped rationale tokens as defined in Equation \ref{eq:token_f1}. 
    
    % Token-F1 $=\frac{1}{N} \sum_{i=1}^{N}\left(2 \times \frac{P_{i} \times R_{i}}{P_{i}+R_{i}}\right)$ \\ where $P_{i}=\frac{\left|S_{i}^{p} \cap S_{i}^{g}\right|}{\left|S_{i}^{p}\right|}$ and $R_{i}=\frac{\left|S_{i}^{p} \cap S_{i}^{g}\right|}{\left|S_{i}^{g}\right|}$ 
    \begin{equation}
        \operatorname{Token-F1} =\frac{1}{N} \sum_{i=1}^{N}\left(2 \times \frac{P_{i} \times R_{i}}{P_{i}+R_{i}}\right)
    \label{eq:token_f1}
    \end{equation}
   
    \begin{equation}
    P_{i}=\frac{\left|S_{i}^{p} \cap S_{i}^{g}\right|}{\left|S_{i}^{p}\right|}, R_{i}=\frac{\left|S_{i}^{p} \cap S_{i}^{g}\right|}{\left|S_{i}^{g}\right|}
    \end{equation}
    
    where $S_i^p$ and $S_i^q$ represent the rationale set of the $i$-th instance provided by the model and human respectively, and $N$ is the number of instance.
    \item \textbf{MAP} measures the consistency of rationales under perturbations.
    
    \begin{equation}
    \operatorname{MAP}=\frac{\frac{1}{i}\sum_{i=1}^{\left|X^{p}\right|}\left(\sum_{j=1}^{i} G\left(x_{j}^{p}, X_{1: i}^{o}\right)\right)}{\left|X^{p}\right|}
    \label{eq:map}
    \end{equation}
    where $X^o$ and $X^p$ represent the sorted rationale token list of the original and perturbed inputs, according to the token important scores assigned by a certain saliency method. $|X^p|$ represents the number tokens of $X^p$. $X^o_{1:i}$ consists of top-$i$ important tokens of $X^o$ . The function $G(x, Y )$ is to determine whether the token $x$ belongs to the list $Y$,where $G(x,Y)=1 \mathbf{if} x\in Y$.
    \item \textbf{Suff \& Comp} are jointly used to evaluate model faithfulness, as defined in Equation \ref{eq:suff}. A faithful rationale should have a low sufficiency score and a high comprehensiveness score.
    \begin{equation}
    \begin{aligned}
    \operatorname { Suff }&=\frac{1}{N} \sum_{i=1}^{N}\left(F\left(x_{i}\right)_{j}-F\left(r_{i}\right)_{j}\right) \\
    \operatorname { Comp }&=\frac{1}{N} \sum_{i=1}^{N}\left(F\left(x_{i}\right)_{j}-F\left(x_{i} \backslash r_{i}\right)_{j}\right)
    \end{aligned}
    \label{eq:suff}
    \end{equation}
    
    where $F(x_i)_j$ represents the prediction probability provided by the model $F$ for the class $j$ on the input $x_i$, $r_i$ represents the rationale of $x_i$, and $x_i \backslash r_i$ represents its non-rationale.

\end{itemize}
\input{table/interpretability_results}
We adopt \textbf{Attention-based (ATT)} \cite{} method to extract rationales based on the predictions, where attention weights based on the specific model architecture are used as important scores. Table \ref{tab:interpretability_results} shows the evaluation results of interpretability from the plausibility and faithfulness. We can observe that compare with BERT, \textit{DeRC} significantly achieve token f1 score improvements of 5\% and 3.94\% on two datasets, respectively. This indicates the model prediction is less misled by shortcuts in datasets.

\begin{table}[h]
\begin{tabular}{lcccc}
\hline
\multicolumn{1}{l|}{\multirow{2}{*}{}} & \multicolumn{2}{c|}{SA}                               & \multicolumn{2}{c}{STS}                               \\ \cline{2-5} 
\multicolumn{1}{l|}{}                  & \multicolumn{1}{c|}{base} & \multicolumn{1}{c|}{DeRC} & \multicolumn{1}{c|}{base} & DeRC                      \\ \hline
alternative dispensable words          & 92.15                     & 92.31                     & 91.60                     & 92.00                     \\ \hline
alternative important words            & 92.25                     & 93.22                     & 90.31                     & 91.53                     \\ \hline
syntax transformation                  & 89.00                     & 89.30                     & 94.87                     & 96.00                     \\ \hline
insert negative words                  & 83.41                     & 85.42                     & 92.00                     & 92.00                     \\ \hline
all types perturbations                & \multicolumn{1}{l}{89.19} & \multicolumn{1}{l}{90.06} & \multicolumn{1}{l}{92.19} & \multicolumn{1}{l}{92.88} \\ \hline
\end{tabular}
\caption{}
\label{tab:robustness}
\end{table}

\paragraph{Model Robustness} We believe that if \textit{DeRC} relies on the semantic understanding of input text to make predictions, its inference ability can be correspondingly improved. To verify this claim, we evaluate the robustness of \textit{DeRC} by using four types of perturbed datas annotated by \citet{wang2022fine}. The results are shown in Table \ref{tab:robustness}. We can observe that \textit{DeRC} achieves higher accuracy than other models, indicating that our proposed framework indeed enhances the robustness of the model.

\paragraph{Impact of Residual Connection} 
To analyze how residual connection take effects for debiasing the top-layer representation, we draw the line of accuracy on MNLI validation set and HANS during training in the Figure \ref{}. 
We
